# Supplementary material for: Vagus nerve stimulation: Laying the groundwork for predictive network-based computer models
Source: arXiv:2406.02729 source file (2024-06-04)
Supplement: Supplementary file 1 [file Supplementary_section_as_separate.pdf]

# Supplementary

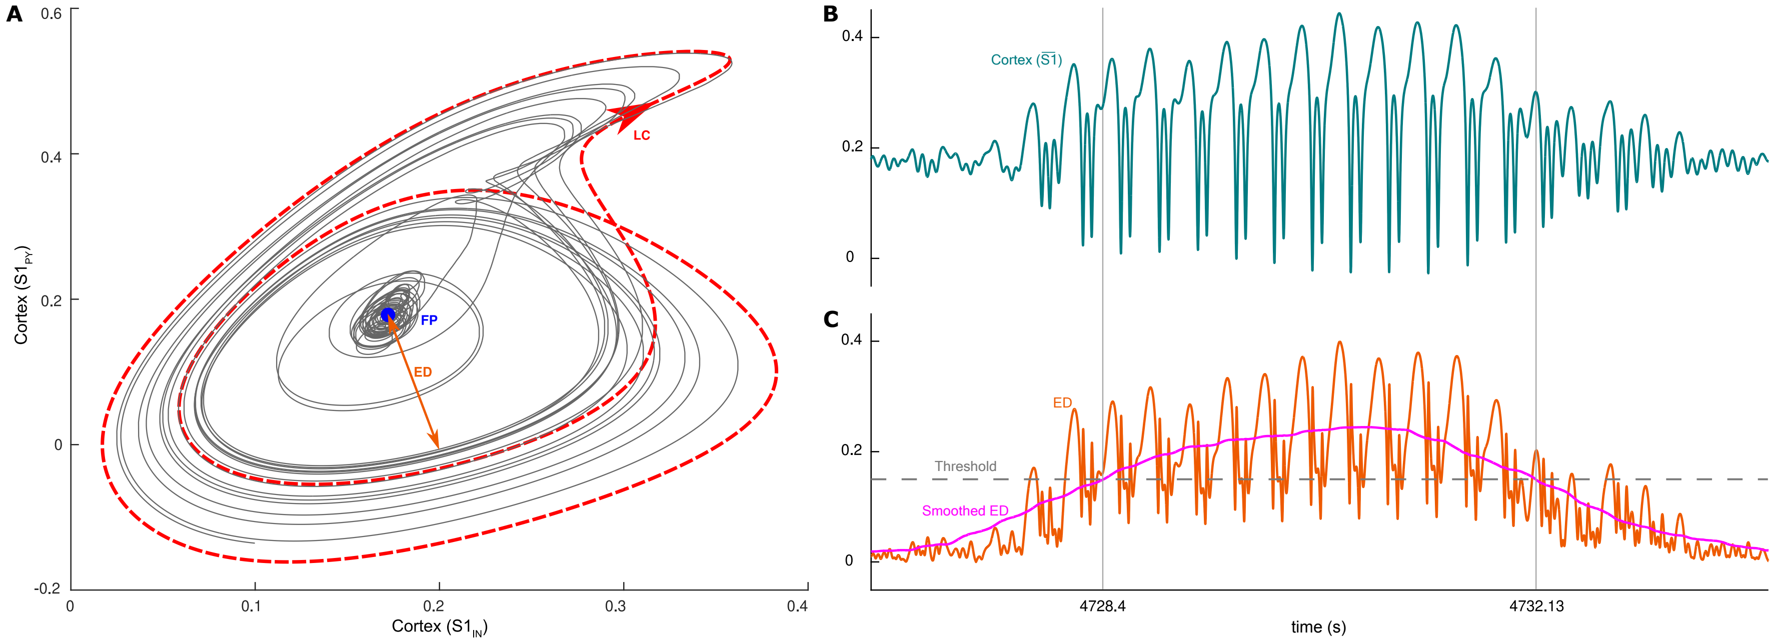


**Figure S0.1: Seizure detection mechanism.** A sample from a run of the stochastic model shown as a phase plot (A) and time series (B,C). The grey line in (A) represents the trajectory of the system in the $S1_{IN}$ - $S1_{PY}$ plane. The red dashed line shows the trajectory of the LC in the deterministic system, while the FP is shown in blue. The mean value of the S1 populations is shown by the blue line in (B), which shows the emergence and resolution of a seizure from normal background activity. The ED between the state of the system and the FP, an example of which is shown by the orange arrow in (A), is plotted against time in (C). A two-second moving mean of the ED is shown in magenta. When this exceeds the threshold of 0.15, shown by the dashed line, the model is determined to be in a seizure state, while values below the threshold are deemed represent normal brain activity. The exact time onset of each seizure episode, as well as its duration, is then stored for later analysis and reconstruction of the local time series as required.

| Connection weights | from: | $S1_{PY}$ | $S1_{IN}$ | TC | RE | INS | $INS_{IN}$ | $ACC_{EX}$ | $ACC_{IN}$ | $PFC_{PY}$ | $PFC_{IN}$ | $Amy_{PY}$ | $Amy_{IN}$ | $Hyp_{PY}$ | $Hyp_{IN}$ | $LoC_{PY}$ | $LoC_{IN}$ | $DRN_{PY}$ | $DRN_{IN}$ | $PB_{PY}$ | $PB_{IN}$ | $NTS_{PY}$ | $STN_{IN}$ |
|---|---|---|---|---|---|---|---|---|---|---|---|---|---|---|---|---|---|---|---|---|---|---|---|
| | to: | | | | | | | | | | | | | | | | | | | | | | |
| Cortex | $S1_{PY}$ | 1.8 | -1.5 | 1 | | | | | | | | | | | | | | | | | | | |
| | $S1_{IN}$ | 4 | | | | | | | | | | | | | | | | | | | | | |
| Thalamus | TC | 3 | | | 0.2* | | | | | | | | | | | | | | | | | | |
| | RE | 3 | | 0.6* | 10.5* | 0.0251 | | | | 0.2431 | | 6.6945 | | | | 0.01 | | | | | | 0.08 | |
| Insula | $INS_{PY}$ | | | 0.0025 | | 1.8 | -1.5 | | | | | 0.4341 | | | | | | | | | | | |
| | $INS_{IN}$ | | | | | 4 | | | | | | | | | | | | | | | | | |
| Anterior Cingulate Gyrus | $ACC_{PY}$ | | | | | | | 1.8 | -1.5 | 0.1399 | | | | 0.2 | | | | | | | | | |
| | $ACC_{IN}$ | | | | | | | 4 | | | | | | | | | | | | | | | |
| Prefrontal Cortex | $PFC_{PY}$ | | | | | | | 0.1399 | | 1.8 | -1.5 | 0.0794 | | | | | | 1 | 0.2 | | | | |
| | $PFC_{IN}$ | | | | | | | | | 4 | | | | | | | | | | | | | |
| Amygdala | $Amy_{PY}$ | | | 6.6945 | | 0.4341 | | | | | | 1.8 | -1.5 | 1 | | 1 | | | | 1 | | 1 | |
| | $Amy_{IN}$ | | | | | | | | | | | 4 | | | | | | | | | | | |
| Hypothalamus | $Hyp_{PY}$ | | | 0.6 | | 1 | | 0.2 | | 3 | | 1 | | 1.8 | -1.5 | | | | | 1 | | 1 | |
| | $Hyp_{IN}$ | | | | | | | | | | | | | 4 | | | | | | | | | |
| Locus Coeruleus | $LoC_{PY}$ | | | | | | | | | | | | | | | 1.8 | -1.5 | | | | | 3 | |
| | $LoC_{IN}$ | | | | | | | | | | | | | | | 4 | | | | | | | |
| Dorsal Raphe Nucleus | $DRN_{PY}$ | | | | | | | | | | | | | | | 1 | | 1.8 | -1.5 | 1 | | | |
| | $DRN_{IN}$ | | | | | | | | | | | | | | | | | 4 | | | | | |
| Parabrachial Nucleus | $PB_{PY}$ | | | | | | | | | | | 1 | | | | 1 | | | | 1.8 | -1.5 | 3 | |
| | $PB_{IN}$ | | | | | | | | | | | | | | | | | | | 4 | | | |
| Nucleus Tractus Solitarius | $NTS_{PY}$ | | | | | | | | | | | | | 0.2 | | | | | | | | 1.8 | |
| | $NTS_{IN}$ | | | | | | | | | | | | | | | | | | | | | 4 | |

**Table S0.1: Connection weights between neuronal populations.** (*Note that connections between TC and RE populations are not included in 'VNSconnectivity.mat' as they are calculated by a different method.)

| | |
|---|---|
| Values of $h$ (the background input of a neuronal population) | |
| $NTS_{PY}$* | -0.9 |
| $NTS_{INH}$** | -0.7 |
| TC | -2.05 |
| RE | -12 |
| all other excitatory populations | -0.35 |
| for all other inhibitory populations | -3.4 |
| Values of $\tau$ (time constant) | |
| All excitatory populations and RE | 26 |
| All other inhibitory populations | 32.5 |
| Standard deviation of noise | 0.72 |

* when fixed during VNS
** when fixed in stochastic versions of the model, with and without VNS

**Table S0.2: Table of other parameters used in the model**

## Hardware and software used.

The simulations were run in MATLAB v2022a, both under Windows 10 Enterprise on an Intel Core i5-9500 CPU @3.00GHz, with 6GB RAM, and running under SLURM on a remote Linux cluster using 44 cores over two Intel Xeon E5-2699 v4 processors (2.2GHz, 55 MB cache) and 128 GB memory across 8 RDIMMs.
